# Supplementary material for: A unified description of Surface Free Energy and Surface Stress
Source: arXiv:1911.02130 ancillary file (2020-03-26)
Supplement: Supplementary file 1 [file SI_v2.pdf]

# Supplemental Material for
# " A unified description of Surface Free Energy and Surface Stress "

Nicodemo Di Pasquale* and Ruslan L. Davidchack

*School of Mathematics and Actuarial Science, University of Leicester, University Rd, Leicester LE1 7RH, UK*

* Email: ndp8@leicester.ac.uk

## S.1. FORM OF THE STRESS TENSOR IN FLUIDS

Let us consider an orthogonal transformation $O \in O(3)$, then, thanks to the isotropy assumption (see Assumption vi in the main paper), we must have $O^T \mathcal{H}(\mathbf{x}) O = \mathcal{H}(\mathbf{x})$ for every point of the system we are considering, where $O^T$ is the transpose of $O$. The former conditions is satisfied only if $\mathcal{H}(\mathbf{x})$ is a multiple, at every point $\mathbf{x}$, of the identity matrix $\mathcal{I}$. It follows that must exist a scalar function of the position that we call $P(\mathbf{x}) : \mathbb{R}^3 \to \mathbb{R}$, and from which we can write $\mathcal{H} = -P(\mathbf{x})\mathcal{I}$. From the fact that the fluid is homogeneous, $\mathcal{H}(\mathbf{x}+\mathbf{t}) = \mathcal{H}(\mathbf{x})$ for any translation $\mathbf{t}$. This condition means that $P(\mathbf{x}) = P(\mathbf{x}+\mathbf{t})$, i.e. $P$ is a scalar constant independent of the position. We identify $P$ with the macroscopic pressure. The reason for the negative sign in front of $P$ comes form the convention of the sign of the stresses which are represented as the negative of the pressure [3]. The liquid is said to be in a hydrostatic state of stress, where the stress tensor has the following form:

$$\mathcal{H} = \begin{bmatrix} \eta_{11} & \eta_{12} & \eta_{13} \\ \eta_{21} & \eta_{22} & \eta_{23} \\ \eta_{31} & \eta_{32} & \eta_{33} \end{bmatrix} = \begin{bmatrix} -\pi_{11} & -\pi_{12} & -\pi_{13} \\ -\pi_{21} & -\pi_{22} & -\pi_{23} \\ -\pi_{31} & -\pi_{32} & -\pi_{33} \end{bmatrix} = \begin{bmatrix} -P & 0 & 0 \\ 0 & -P & 0 \\ 0 & 0 & -P \end{bmatrix} \tag{S.1}$$

where we indicated the components of the stress tensor as $\eta_{ij}$, the components of the pressure tensor as $\pi_{ij}$ with the convention that the pressure is equal to the negative of the stress.

## S.2. MOLECULAR DYNAMICS RESULTS

The density, $\rho$, at zero temperature is obtained by minimizing the energy of a fcc crystal. Thus determined value of $\rho$ is reported in Table S.1 and is consistent with the value reported in [1]. The density at finite temperature is obtained by relaxing the initial crystal structure in a simulation in the NVT ensemble followed by a simulation in the NPT ensemble at $P = 0$. We used the Nose-Hoover thermostat in both cases and the Nose-Hoover barostat for NPT calculations. A summary of the results is reported in Table S.1. From the density, the size of the unit cell of the fcc crystal, $a$, can be obtained as: $a = (4/\rho)^{\frac{1}{3}}$.

| T | $\rho$ |
|---|---|
| $\epsilon$ | $\sigma^{-3}$ |
| 0 | 1.07309 |
| 0.1 | 1.05604(4) |
| 0.2 | 1.03843(7) |
| 0.3 | 1.01987(6) |

**TABLE S.1:** Density ($\rho$) for all the temperatures considered

The unit cell parameter depends on the temperature, $a(T)$. However, to reduce the notation we will drop the dependence where there is no risk of confusion. The size of the box $(L_x, L_y, L_z)$ and number of particles $N$ for different orientations for the cleaving TI calculations are as follows:

(100) : $L_x = L_y = 9a$, $L_z = 20a$, $N = 6480$

(110) : $L_x = 6\sqrt{2}a$, $L_y = 9a$, $L_z = 12\sqrt{2}a$, $N = 5184$

(111) : $L_x = 5.5\sqrt{2}a$, $L_y = 3\sqrt{6}a$, $L_y = 12\sqrt{3}a$, $N = 4752$

The size of the box for the slab calculation is different. We used a bigger box in order to reduce the finite size effects that can be more pronounced in the calculation of the stress in the box. We have in this case:

(100) : $L_x = L_y = L_z = 16a$, $N = 16384$

(110) : $L_x = 12\sqrt{2}a$, $L_y = 16a$, $L_z = 11\sqrt{2}a$, $N = 16896$

(111) : $L_x = 11.5\sqrt{2}a$, $L_y = 13\sqrt{1.5}a$, $L_x = 9\sqrt{3}a$, $N = 16146$

In wells model (see Section 6.1.1 of the main paper) there are two parameters than need to be fixed to perform the simulations: the depth of the well $d_w$ and the cut-off radius for the attraction of the wells (see Equation (56)). In this work we define these two parameters as follows:

- $d_w = 6\,\epsilon$, which is approximately the energy per particle of a fcc crystal at the melting temperature $T = 0.617\epsilon$ [2]
- $r_w(T) = \frac{\sqrt{2}}{4} a(T)\sigma$ which represents the nearest neighbour distance in the fcc crystal

While the depth of the well $d_w$ is the same for all the systems at all temperatures, the parameter $r_w$ depends on $T$ through the unit cell parameter $a(T)$.

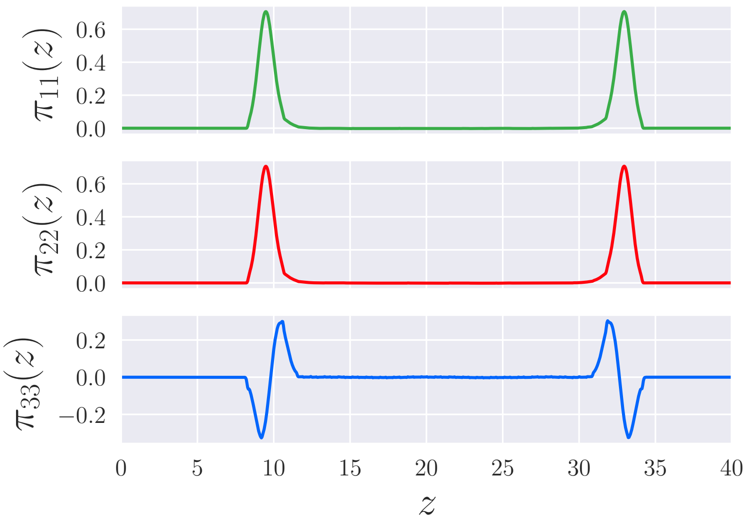


**FIG. S.1:** Pressure profile for fcc111 at temperature T=0.2 $\epsilon$ in the three spatial directions

### A. Calculation of the derivative $\frac{\mathrm{d}\gamma^u}{\mathrm{d}u}$

The derivative $\frac{\mathrm{d}\gamma^u}{\mathrm{d}u}$ is calculated numerically by fitting the results of the calculations at different strain with a straight line, $\gamma = a_0 + a_1 u$, and a parabola, $\gamma = b_0 + b_1 u + b_2 u^2$. The coefficients $a_0$, $a_1$ and $b_0$, $b_1$, $b_2$ are estimated using linear least square regression. The derivative $\frac{\mathrm{d}\gamma^u}{\mathrm{d}u}$ is then given by the coefficient $a_1$ or the coefficient $b_1$. We considered two different functions to check that $a_1 = b_1$ (within the error bars). This consistency check ensure that all the points we considered could be

effectively fitted by a straight line and the slope of this straight line represents the quantity we need

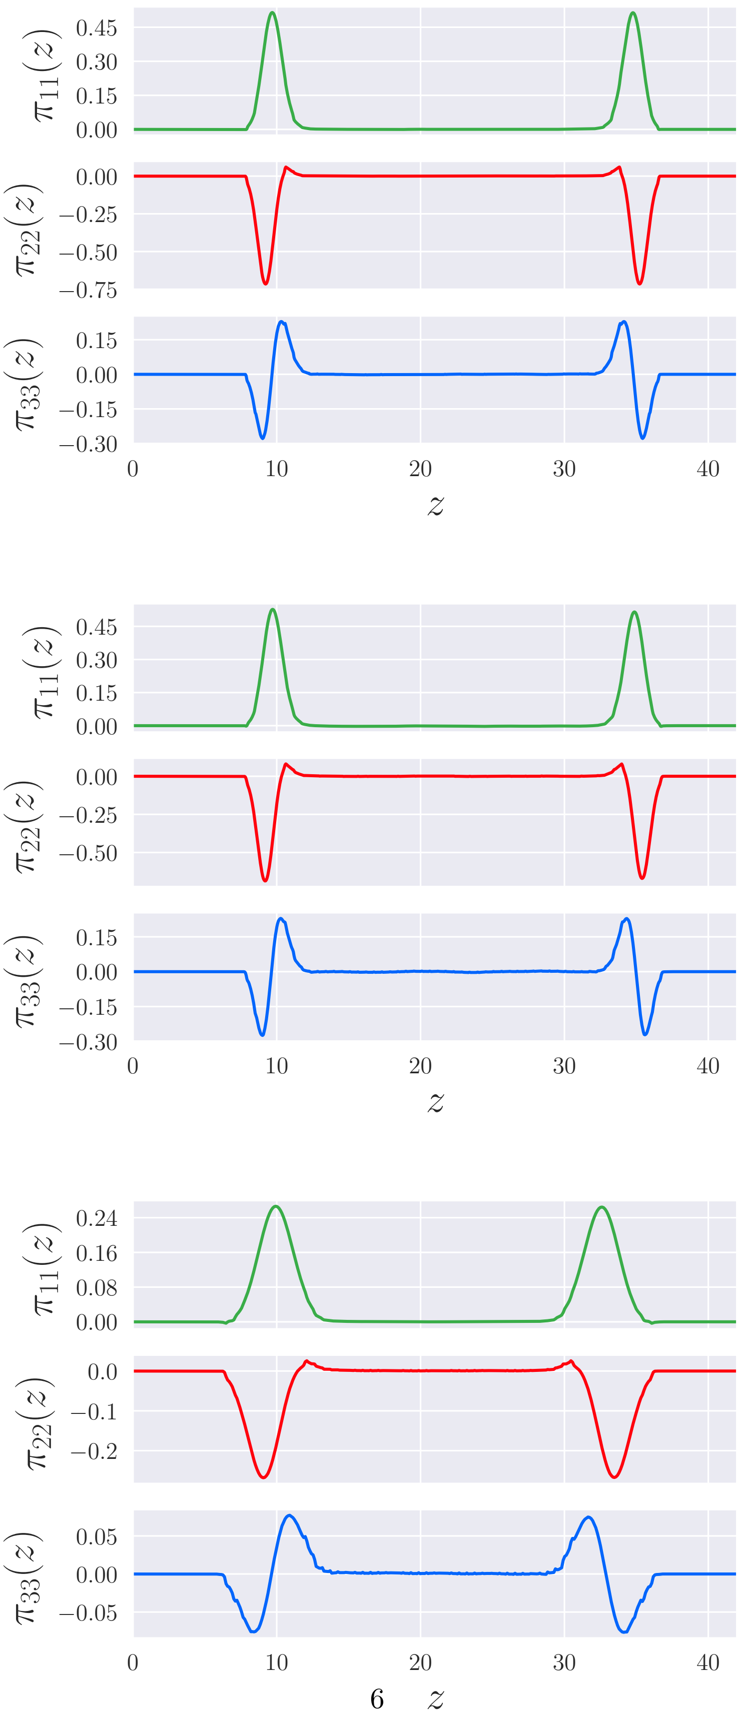




**FIG. S.2:** From top to bottom: pressure profile for a (110) slab at temperatures T=0.1, 0.2, 0.3 $\epsilon$ in the three spatial directions.

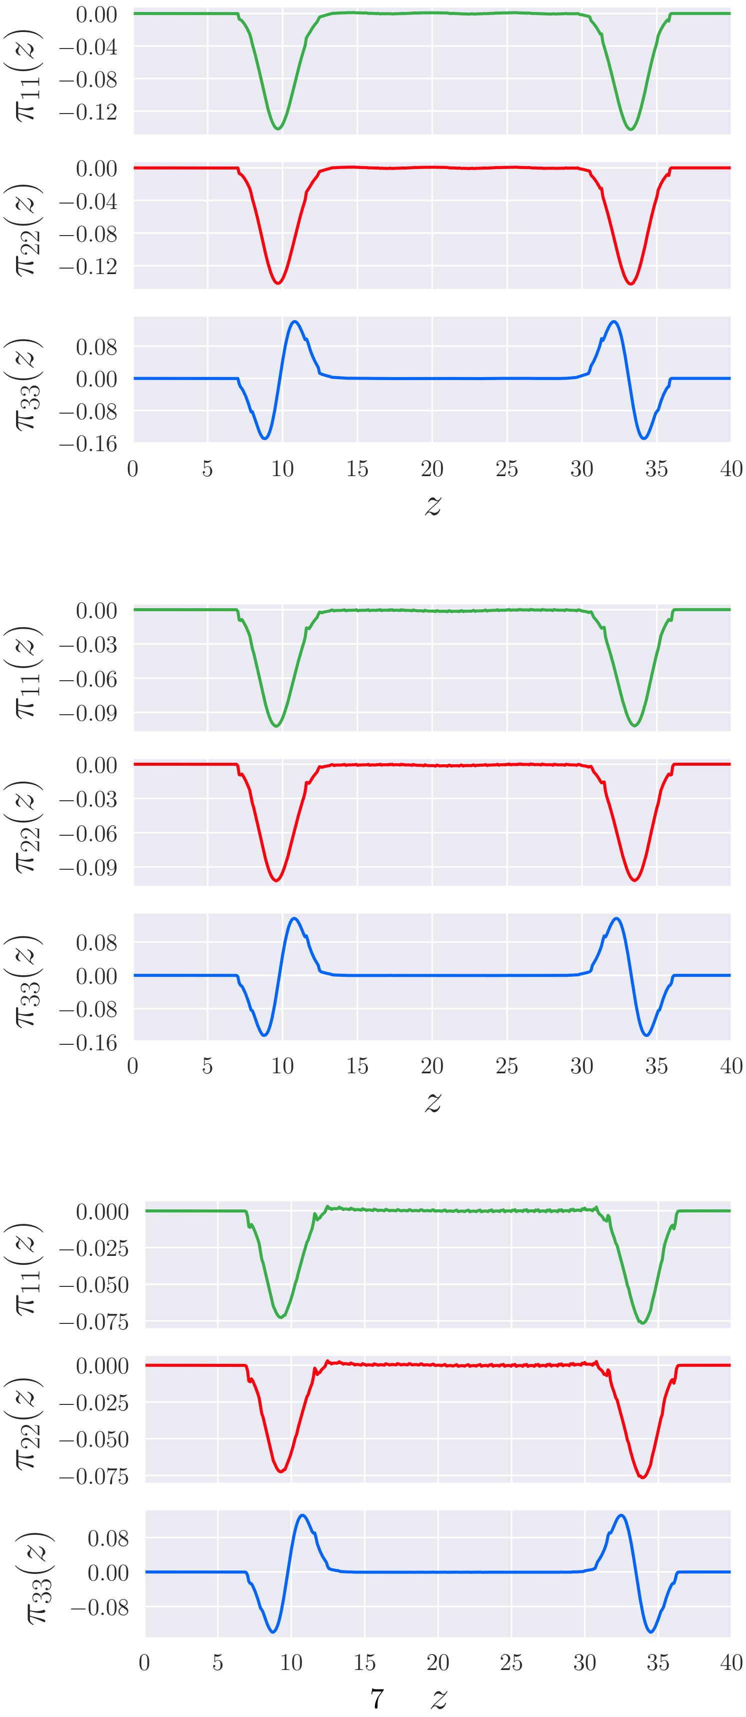




**FIG. S.3:** From top to bottom: pressure profile for (100) slab at temperatures T=0.1, 0.2, 0.3 $\epsilon$ in the three spatial directions.

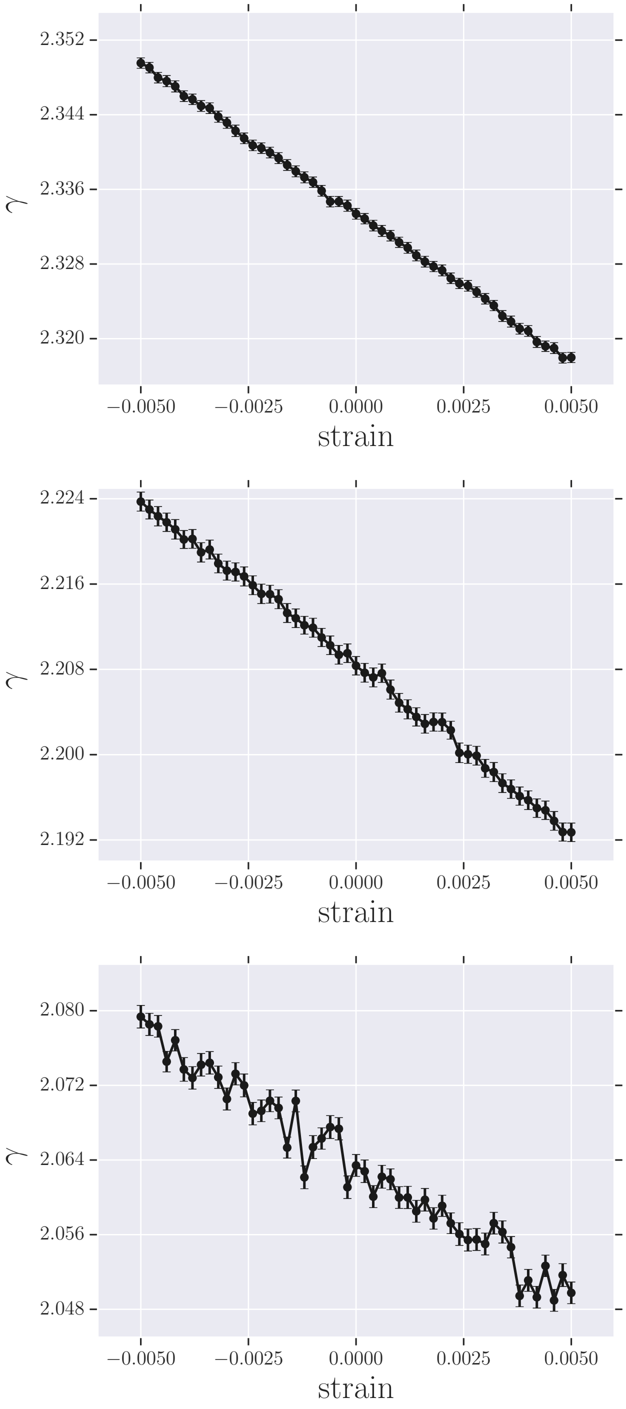


**FIG. S.4:** From top to bottom, surface free energy $\gamma$ as function of the strain rate in the $x$-direction for (110) surface at three temperatures, T=0.1, 0.2, 0.3 $\epsilon$.

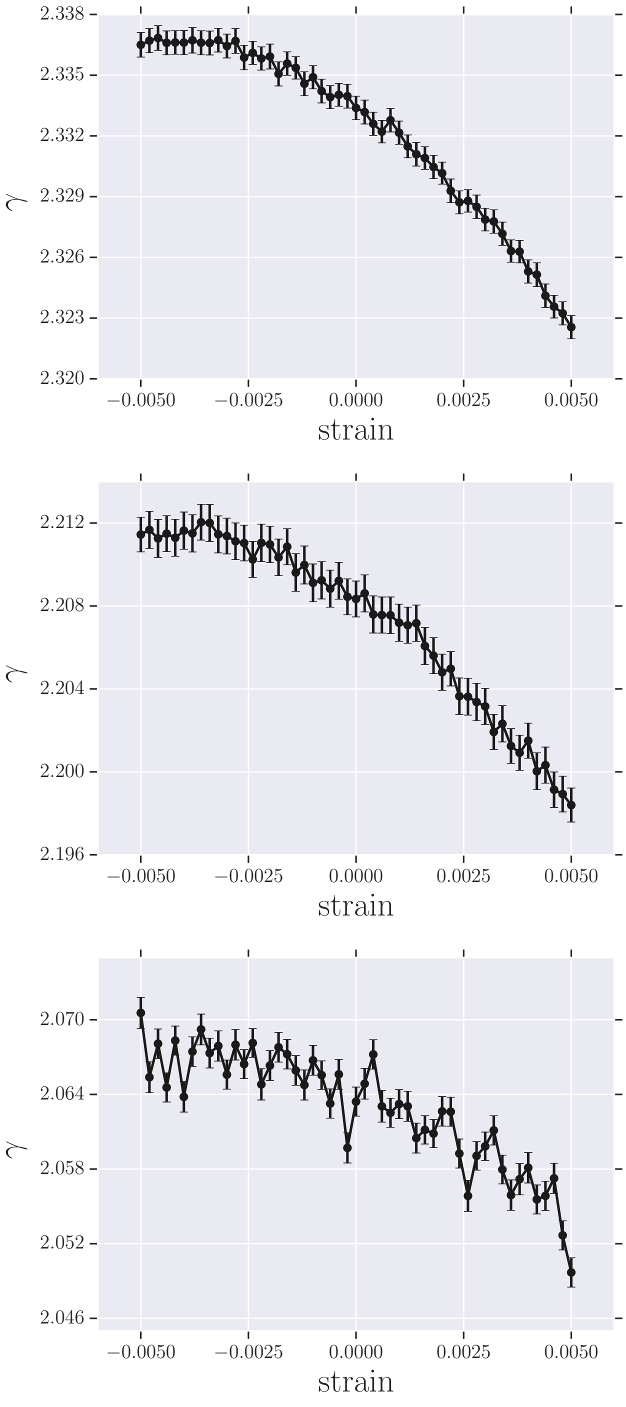


**FIG. S.5:** From top to bottom, surface free energy $\gamma$ as function of the strain rate in the $y$-direction for (110) surface at three temperatures, T= 0.1, 0.2, 0.3 $\epsilon$.

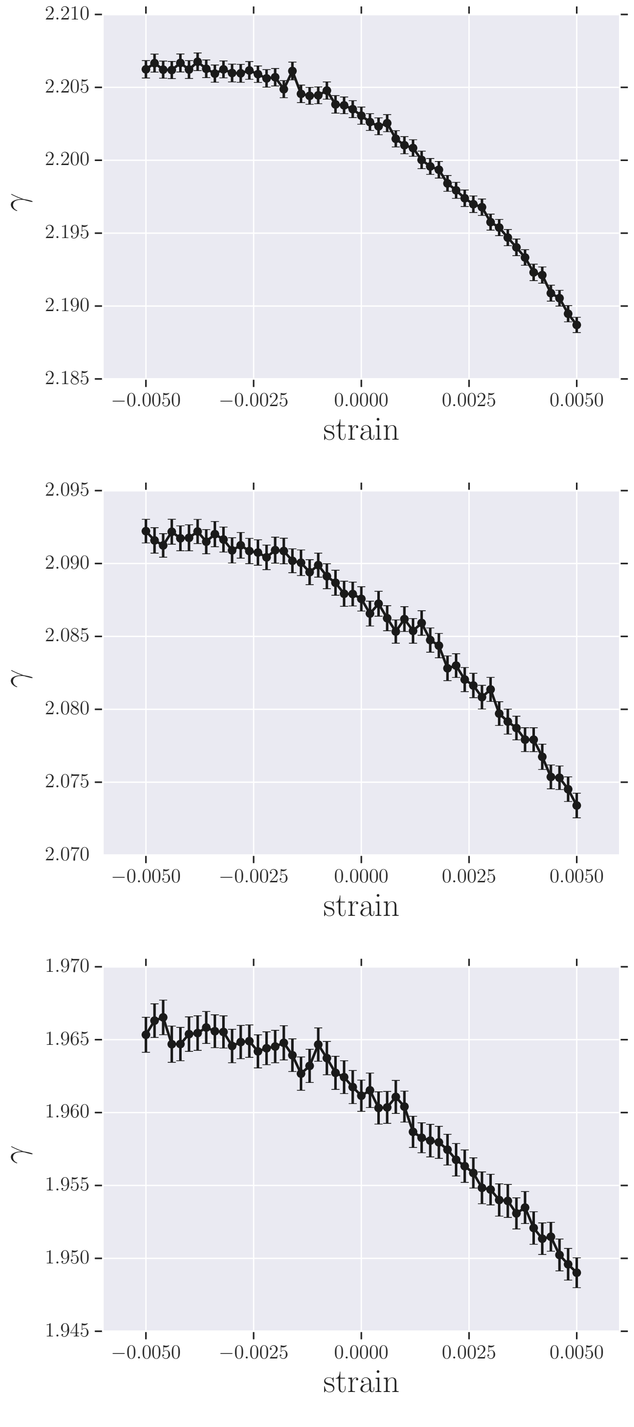


**FIG. S.6:** From top to bottom, surface free energy $\gamma$ as function of the strain rate in the $x$-direction for (100) surface at three temperatures, T=0.1, 0.2, 0.3 $\epsilon$. Where not shown, error bars are smaller than the size of the symbols.

| (111) | | | | |
|---|---|---|---|---|
| T<br>($\epsilon$) | $\gamma$<br>($\epsilon\sigma^{-2}$) | $\frac{\partial\gamma}{\partial u_{22}}$<br>($\epsilon\sigma^{-2}$) | $f_{22}$<br>($\epsilon\sigma^{-2}$) | $\gamma + \frac{\partial\gamma}{\partial u_{22}}$<br>($\epsilon\sigma^{-2}$) |
| 0.1 | 2.0953(6) | −3.00(3) | −0.9235(4) | −0.91(3) |
| 0.2 | 1.9911(9) | −2.91(5) | −0.906(5) | −0.92(5) |
| 0.3 | 1.880(2) | −2.73(6) | −0.923(8) | −0.85(6) |

**TABLE S.2:** Numerical value of different terms in the Shuttleworth equation (see Equation (37)) for (111) surface with strain applied in the $y$-direction.

| (100) | | | | | | |
|---|---|---|---|---|---|---|
| T | $\gamma$ | $\frac{\partial\gamma}{\partial u_{11}}$ | $f_{11}$ | $\gamma+\frac{\partial\gamma}{\partial u_{11}}$ | $\Delta\mathfrak{v}^0$ | $\Delta\mathfrak{s}^0$ |
| ($\epsilon$) | ($\epsilon\sigma^{-2}$) | ($\epsilon\sigma^{-2}$) | ($\epsilon\sigma^{-2}$) | ($\epsilon\sigma^{-2}$) | ($\epsilon$) | |
| 0.1 | 2.2031(6) | −1.73(3) | 0.378(5) | 0.47(3) | 2.2953(3) | 0.922(7) |
| 0.2 | 2.0876(8) | −1.81(4) | 0.267(2) | 0.28(4) | 2.2856(4) | 0.990(5) |
| 0.3 | 1.961(1) | −1.68(5) | 0.188(3) | 0.28(5) | 2.2970(8) | 1.120(4) |

**TABLE S.3:** Numerical value of different terms in the Shuttleworth equation (see Equation (37)) for (100) surface with strain applied in the $x$-direction. $\Delta\mathfrak{s}^0$ represents the entropy term calculated from equation Equation (64) in the main paper.

| (100) | | | | |
|---|---|---|---|---|
| T | $\gamma$ | $\frac{\partial\gamma}{\partial u_{22}}$ | $f_{22}$ | $\gamma + \frac{\partial\gamma}{\partial u_{22}}$ |
| $(\epsilon)$ | $(\epsilon\sigma^{-2})$ | $(\epsilon\sigma^{-2})$ | $(\epsilon\sigma^{-2})$ | $(\epsilon\sigma^{-2})$ |
| 0.1 | 2.2031(6) | −1.73(3) | 0.377(2) | 0.48(3) |
| 0.2 | 2.0871(9) | −1.77(4) | 0.267(2) | 0.32(4) |
| 0.3 | 1.962(1) | −1.72(6) | 0.188(3) | 0.25(6) |

**TABLE S.4:** Numerical value of different terms in the Shuttleworth equation (see Equation (37)) for (100) surface with strain applied in the $y$-direction.

| (110) | | | | | | |
|---|---|---|---|---|---|---|
| T | $\gamma$ | $\frac{\partial\gamma}{\partial u_{11}}$ | $f_{11}$ | $\gamma + \frac{\partial\gamma}{\partial u_{11}}$ | $\Delta\mathfrak{v}^0$ | $\Delta\mathfrak{s}^0$ |
| $(\epsilon)$ | $(\epsilon\sigma^{-2})$ | $(\epsilon\sigma^{-2})$ | $(\epsilon\sigma^{-2})$ | $(\epsilon\sigma^{-2})$ | $(\epsilon)$ | |
| 0 | 2.452284 | −3.300510 | −0.848423 | −0.848226 | 2.452284 | - |
| 0.1 | 2.3334(6) | −3.19(3) | −0.846(2) | −0.85(3) | 2.4302(2) | 0.968(7) |
| 0.2 | 2.2083(9) | −3.12(5) | −0.898(3) | −0.91(5) | 2.4194(4) | 1.056(5) |
| 0.3 | 2.063(2) | −2.87(6) | −0.783(8) | −0.81(6) | 2.485(2) | 1.41(1) |

**TABLE S.5:** Numerical value of different terms in the Shuttleworth equation (see Equation (37)) for (110) surface with strain applied in the $x$-direction. $\Delta\mathfrak{s}^0$ represents the entropy term calculated from equation Equation (64) in the main paper.

| 110 | | | | |
|---|---|---|---|---|
| T | $\gamma$ | $\frac{\partial\gamma}{\partial u_{22}}$ | $f_{22}$ | $\gamma + \frac{\partial\gamma}{\partial u_{22}}$ |
| $(\epsilon)$ | $(\epsilon\sigma^{-2})$ | $(\epsilon\sigma^{-2})$ | $(\epsilon\sigma^{-2})$ | $(\epsilon\sigma^{-2})$ |
| 0.1 | 2.3334(6) | −1.41(3) | 0.922(1) | 0.92(3) |
| 0.2 | 2.2083(9) | −1.35(4) | 0.823(2) | 0.86(4) |
| 0.3 | 2.063(2) | −1.38(6) | 0.69(2) | 0.68(6) |

**TABLE S.6:** Numerical value of different terms in the Shuttleworth equation (see Equation (37)) for (110) surface with strain applied in the $y$-direction.

## S.3. DERIVATION OF SOME OF THE EQUATIONS IN THE MAIN TEXT

### A. Equation (10)

$$\begin{aligned}
\mathrm{d}\mathcal{W} &= \int\int\int_{V^\sigma} \left(\eta^\sigma_{ij}(z)u_{ij}\right)\mathrm{d}x\mathrm{d}y\mathrm{d}z \\
&= \int\int\int_{V^\sigma} (\varepsilon_{ij}(z)u_{ij})\mathrm{d}x\mathrm{d}y\mathrm{d}z + \int\int\int \left(\eta^\alpha_{ij}u_{ij}\right)\mathrm{d}x\mathrm{d}y\mathrm{d}z \\
&= \int\int\int_{V^\sigma} (\varepsilon_{ij}(z)u_{ij})\mathrm{d}x\mathrm{d}y\mathrm{d}z = \mathrm{d}\mathcal{W}^A
\end{aligned} \tag{S.2}$$

### B. Equation (11)

$$\begin{aligned}
\mathrm{d}\mathcal{W}^A &= \int\int\int_{V^\sigma} \left(\varepsilon^\sigma_{ij}(z)u_{ij}\right)\mathrm{d}x\mathrm{d}y\mathrm{d}z \\
&= \int\int\int_{V^\sigma} \mathrm{d}x\mathrm{d}y\mathrm{d}z\,(-\pi_{11}(z)u_{11}) + \int\int\int_{V^\sigma} \mathrm{d}x\mathrm{d}y\mathrm{d}z\,(-\pi_{22}(z)u_{22}) \\
&= A\int_0^h \mathrm{d}z\,(-\pi_{11}(z)u_{11}) + A\int_0^h \mathrm{d}z\,(-\pi_{22}(z)u_{22}) \\
&= Af_{11}u_{11} + Af_{22}u_{22}
\end{aligned} \tag{S.3}$$

### C. Equation (19)

$$\begin{aligned}
\mathrm{d}\mathcal{W} &= \int\int\int_{V^\sigma} \left(\eta^\sigma_{ij}(z)u_{ij}\right)\mathrm{d}x\mathrm{d}y\mathrm{d}z \\
&= \int\int\int_{V^\sigma} \left(\varepsilon^\sigma_{ij}(z)u_{ij}\right)\mathrm{d}x\mathrm{d}y\mathrm{d}z + \int\int\int_{V^\sigma} \left(\eta^\alpha_{ij}u_{ij}\right)\mathrm{d}x\mathrm{d}y\mathrm{d}z \\
&= A\int_{-\infty}^{+\infty} \mathrm{d}z\,(P-\pi_{11}(z))\,u_{11} + A\int_{-\infty}^{+\infty} \mathrm{d}z\,(P-\pi_{22}(z))\,u_{22} - PV^\sigma(u_{11}+u_{11}+u_{33}) \\
&= \mathrm{d}A\int_{-\infty}^{+\infty} \mathrm{d}z\,(P-(\pi(z))) - P\mathrm{d}V^\sigma = \\
&= \mathrm{d}\mathcal{W}^A + \mathrm{d}\mathcal{W}^M
\end{aligned} \tag{S.4}$$

where we used the fact that the change of volume due to strain is $\mathrm{d}V = V(u_{11}+u_{22}+u_{33})$, the change of surface area is $\mathrm{d}A = A(u_{11}+u_{22})$, and the fact that $\pi_{11}(z) = \pi_{22}(z) = \pi(z)$.

### D. Equation (28)

$$\begin{aligned}
\mathrm{d}\mathcal{W} &= \int\int\int_{V^\sigma} \left(\eta^\sigma_{ij}(z)u_{ij}\right)\mathrm{d}x\mathrm{d}y\mathrm{d}z \\
&= \int\int\int_{V^\sigma} \left(\varepsilon^\sigma_{ij}(z)u_{ij}\right)\mathrm{d}x\mathrm{d}y\mathrm{d}z + \int\int\int_{V^\sigma} \left(\eta^\alpha_{ij}u_{ij}\right)\mathrm{d}x\mathrm{d}y\mathrm{d}z \\
&= A\int_{-\infty}^{+\infty}\mathrm{d}z\,(P-\pi_{11}(z))\,u_{11} + A\int_{-\infty}^{+\infty}\mathrm{d}z\,(P-\pi_{22}(z))\,u_{22} + A\int_{-\infty}^{+\infty}\mathrm{d}z\,(-\pi_{12}(z))\,u_{12} \\
&\quad + A\int_{-\infty}^{+\infty}\mathrm{d}z\,(-\pi_{21}(z))\,u_{21} - PV^\sigma(u_{11}+u_{22}+u_{33}) \\
&= \mathrm{d}\mathcal{W}^A + \mathrm{d}\mathcal{W}^M
\end{aligned} \tag{S.5}$$

where $PV^\sigma(u_{11}+u_{22}+u_{33}) = P\mathrm{d}V^\sigma$ using the fact that the change of volume due to strain is $\mathrm{d}V = V(u_{11}+u_{22}+u_{33})$.

### E. Derivative of the SFE

We have

$$\begin{aligned}
\frac{\mathrm{d}\gamma^u}{\mathrm{d}u} &= \frac{\partial}{\partial u}\left(\frac{\mathcal{U}_s^{TOT,u} - \mathcal{U}_b^{TOT,u}}{A^u}\right) \\
&= -\frac{\mathcal{U}_s^{TOT,u} - \mathcal{U}_b^{TOT,u}}{A^0(1+u)^2} + \frac{1}{A^u}\frac{\partial}{\partial u}\left(\mathcal{U}_s^{TOT,u} - \mathcal{U}_b^{TOT,u}\right) \\
&= -\frac{\gamma^u}{(1+u)} + \frac{1}{A^u}\frac{\partial}{\partial u}\left(\mathcal{U}_s^{TOT,u} - \mathcal{U}_b^{TOT,u}\right)
\end{aligned} \tag{S.6}$$

Now, let us calculate the derivative of the potential (in either slab or bulk geometry) with respect the strain $u$.

$$\frac{\partial\mathcal{U}^{TOT,u}}{\partial u} = \sum_i\sum_{j>i}\frac{\partial}{\partial u}U\left(|\hat{\mathbf{r}}_l - \hat{\mathbf{r}}_n|\right) = \sum_l\sum_{n>l}U'\left(\hat{r}_{ln}\right)\frac{\partial\hat{r}_{ln}}{\partial u} \tag{S.7}$$

where $U'(r)$ denotes the derivative of the function $U(r)$ with respect to its (scalar) argument and $\hat{\mathbf{r}}$ represents the point $\mathbf{r}$ in the strained configuration (see end of Section 2 of the main paper). The

last term we need to expand is the derivative $\frac{\partial \hat{r}_{ln}}{\partial u}$:

$$
\begin{aligned}
\frac{\partial \hat{r}_{ln}}{\partial u} &= \frac{\partial}{\partial u}\left((x_l(1+u) - x_n(1+u))^2 + (y_l - y_n)^2 + (z_l - z_n)^2\right)^{\frac{1}{2}} \\
&= \frac{(x_l - x_n)^2(1+u)}{\left((x_l(1+u) - x_n(1+u))^2 + (y_l - y_n)^2 + (z_l - z_n)^2\right)^{\frac{1}{2}}} \\
&= \frac{(x_l - x_n)^2(1+u)}{\hat{r}_{ln}} = \frac{x_{ln}^2(1+u)}{\hat{r}_{ln}},
\end{aligned}
\tag{S.8}
$$

where $x_{ln} = x_l - x_n$.

The derivative is evaluated at $u = 0$, so that

$$
\begin{aligned}
\left(\frac{\mathrm{d}\gamma^u}{\mathrm{d}u}\right)_{u=0} &= \left[-\frac{\gamma^u}{(1+u)} + \frac{1}{A^u}\left(\sum_l \sum_{n>l} U'\left(\hat{r}_{ln}\right)\frac{x_{ln}^2(1+u)}{\hat{r}_{ln}}\right)_s - \frac{1}{A^u}\left(\sum_l \sum_{n>l} U'\left(\hat{r}_{ln}\right)\frac{x_{ln}^2(1+u)}{\hat{r}_{ln}}\right)_b\right]_{u=0} \\
&= -\gamma^0 + \frac{1}{A^0}\sum_l \sum_{n>l}\left[\left(U'\left(r_{ln}\right)\frac{x_{ln}^2}{r_{ln}}\right)_s - \left(U'\left(r_{ln}\right)\frac{x_{ln}^2}{r_{ln}}\right)_b\right] \\
&= -\gamma^0 + \frac{1}{A^0}\sum_l \sum_{n>l}\left[\left(x_{ln}F_{ln}^1\right)_b - \left(x_{ij}F_{ln}^1\right)_s\right]
\end{aligned}
\tag{S.9}
$$

where we recognise that $-U'(r_{ln})\frac{x_{ln}}{r_{ln}} = F_{ln}^1$ is the $x$ component of the force between particles $i$ and $j$. Note that we group the terms in the two double summations together because we assume that the slab and bulk geometries contain the same atoms, with periodic boundary conditions in all directions for the bulk and only in $x$ and $y$ directions for the slab.

### F. Broughton-Gilmer modified Lennard-Jones Potential

$$
U(r_{ln}) = \begin{cases}
4\epsilon\left(\left(\frac{\sigma}{r_{ln}}\right)^{12} - \left(\frac{\sigma}{r_{ln}}\right)^6\right) + C_1, \text{ if } r_{ln} \leq 2.3\sigma \\
C_2\left(\frac{\sigma}{r_{ln}}\right)^{12} + C_3\left(\frac{\sigma}{r_{ln}}\right)^6 + C_4\left(\frac{r_{ln}}{\sigma}\right)^2 + C_5, \text{ if } r_{ln} \leq 2.5\sigma \\
0, \ r_{ln} \geq 2.5\sigma
\end{cases}
\tag{S.10}
$$

where $r_{ln} = |\mathbf{r}_l - \mathbf{r}_n|$ for each couple of atoms $l, n$ in the system, and $C_1, C_2, C_3, C_4, C_5$ are constants (we used the values reported in [2]).

### G. Derivative of BG Potential with respect $z_w$

The derivative of the BG potential (which includes now also the dependence on $z_w$) is:

$$\begin{aligned}\frac{\partial}{\partial z_w} U\left(r_{ln}; z_w\right) &= \begin{cases} 4\varepsilon\left[-\frac{12\sigma^{12}}{(r_{ln})^{13}} + \frac{6\sigma^6}{(r_{ln})^7}\right]\frac{\partial r_{ln}}{\partial z_w}, \text{ if } r_{ln} \leq 2.3\sigma \\ \left[-12C_2\frac{\sigma^{12}}{(r_{ln})^{13}} - 6C_3\frac{\sigma^6}{(r_{ij})^6} + 2C_4\frac{r_{ln}}{\sigma^2}\right]\frac{\partial r_{ln}}{\partial z_w}, \text{ if } r_{ln} \leq 2.5\sigma \end{cases} \\ &= \frac{\partial r_{ln}}{\partial z_w}\frac{\partial}{\partial r_{ln}} U\left(|\mathbf{r}_l - \mathbf{r}_n|\right). \end{aligned} \tag{S.11}$$

Now,

$$\begin{aligned}\frac{\partial r_{ln}}{\partial z_w} &= \frac{\partial}{\partial z_w}\left[\sqrt{(x_l-x_n)^2+(y_l-y_n)^2+(z_l-(z_n+z_w))^2}\right] \\ &= \frac{1}{\sqrt{(x_l-x_n)^2+(y_l-y_n)^2+(z_l-(z_n+z_w))^2}}(z_l-(z_n+z_w))\end{aligned} \tag{S.12}$$

Now, putting everything together:

$$\frac{\partial}{\partial z_w}U\left(r_{ln}; z_w\right) = -\frac{(z_l-(z_n+z_w))}{r_{ln}}\frac{\partial}{\partial r_{ln}}U\left(r_{ln}\right) = F^z_{ln}\left(z_w\right) \tag{S.13}$$

### H. Equation (53)

By using Equations (S.7) to (S.9) we can write:

$$\begin{aligned} f(u) &= \frac{1}{uA^0}\int_0^u \left\langle \mathrm{d}\nu \left(\sum_l\sum_{n>l} U'\left(\hat{r}_{ln}\right)\frac{x_{ln}^2(1+\nu)}{\hat{r}_{ln}}\right)_s - \left(\sum_l\sum_{n>l} U'\left(\hat{r}_{ln}\right)\frac{x_{ln}^2(1+\nu)}{\hat{r}_{ln}}\right)_b\right\rangle_\nu \\ &= \frac{1}{uA^0}\int_0^u \left\langle \mathrm{d}\nu \left(\sum_l\sum_{n>l} U'\left(\hat{r}_{ln}\right)\frac{x_{ln}(x_l(1+\nu)-x_n(1+\nu))}{\hat{r}_{ln}}\right)_\nu \right. \\ &\qquad \left. - \left(\sum_l\sum_{n>l} U'\left(\hat{r}_{ln}\right)\frac{x_{ln}(x_l(1+\nu)-x_n(1+\nu))}{\hat{r}_{ln}}\right)_b\right\rangle_\nu \\ &= \frac{1}{uA^0}\int_0^u \mathrm{d}\nu \left\langle \left(\frac{1}{2}Nk_B\mathcal{T} + \sum_l\sum_{n>l}\left(x_{ln}\hat{F}^1_{ln}(\nu)\right)_b\right) - \left(\frac{1}{2}Nk_B\mathcal{T} + \sum_l\sum_{n>l}\left(x_{ln}\hat{F}^1_{ln}(\nu)\right)_s\right)\right\rangle_\nu \\ &= \frac{1}{uA^0}\int_0^u \frac{\mathrm{d}\nu}{(1+\nu)} \left\langle \left(\frac{1}{2}Nk_B\mathcal{T} + \sum_l\sum_{n>l}\left(\hat{x}_{ln}\hat{F}^1_{ln}(\nu)\right)_b\right) - \left(\frac{1}{2}Nk_B\mathcal{T} + \sum_l\sum_{n>l}\left(\hat{x}_{ln}\hat{F}^1_{ln}(\nu)\right)_s\right)\right\rangle_\nu \end{aligned}$$

where $\hat{F}^1_{ln}(\nu)$ is the $x$-component of the force in the strained system identified by $\nu$, and $x_{ln} = \hat{x}_{ln}/(1+\nu)$ where $\hat{x}_{ln}$ represents the difference in the $x$ coordinate between atom $l$ and atom $n$ in the strained configuration. We defined the instantaneous temperature $\frac{1}{2}Nk_B\mathcal{T} = \sum_l m_l v_l v_l$, with

$m_l$ mass of the atom $l$ and $v_l$ the x-component of the velocity of the atom $l$. We used the fact that the temperature, and therefore the ensemble averaged kinetic energy, does not depend from the system configuration (i.e. slab or bulk).

### I. Equation (45)

$$\begin{aligned} uA^0 f &= -A^0\gamma^0 + A^u \left(\gamma^0 + \left(\frac{\mathrm{d}\gamma^u}{\mathrm{d}u}\right)_{u=0} u\right) \\ &= -A^0\gamma^0 + A^0(1+u)\left(\gamma^0 + \left(\frac{\mathrm{d}\gamma^u}{\mathrm{d}u}\right)_{u=0} u\right) \\ &= uA^0\gamma^0 + uA^0\left(\frac{\mathrm{d}\gamma^u}{\mathrm{d}u}\right)_{u=0} \end{aligned} \tag{S.14}$$

from which we deduce that:

$$f = \gamma^0 + \left(\frac{\mathrm{d}\gamma^u}{\mathrm{d}u}\right)_{u=0}. \tag{S.15}$$

### J. Off-Diagonal terms of the Shuttleworth Equation

If $u$ represents the off-diagonal strain (i.e. $u = u_{12} = u_{21}$) then the deformation of the surface results only in the change of shape without changing the area, i.e. $A^u = A^0$. In this case we can write (e.g. for $u = u_{12}$):

$$uA^0 f_{12} = -A^0\gamma^0 + A^0\left(\gamma^0 + \left(\frac{\mathrm{d}\gamma^u}{\mathrm{d}u}\right)_{u=0} u\right) = uA^0\left(\frac{\mathrm{d}\gamma^u}{\mathrm{d}u}\right)_{u=0}. \tag{S.16}$$

from which

$$f_{12} = \left(\frac{\mathrm{d}\gamma^u}{\mathrm{d}u}\right)_{u=0} \tag{S.17}$$

---


[1] Broughton, J. Q. and G. H. Gilmer (1983). Molecular dynamics investigation of the crystal–fluid interface. i. bulk properties. *The Journal of chemical physics 79*(10), 5095–5104.

[2] Davidchack, R. L. and B. B. Laird (2003). Direct calculation of the crystal–melt interfacial free energies for continuous potentials: Application to the Lennard-Jones system. *Journal of Chemical Physics 118*(16), 7651–7657.

[3] Note1. This derivation does not make any other assumption on $P$, but to be identified with the macroscopic pressure, we need $P$ to be strict positive.
